# Supplementary material for: Magnetic field robust high quality factor NbTiN superconducting microwave resonators
Source: arXiv:2112.08296 ancillary file (2021-12-15)
Supplement: Supplementary file 1 [file Supplements-resonators.pdf]

# Supplementary Material - Magnetic field robust high quality factor NbTiN superconducting microwave resonators

M. Müller,[1,2,a)] T. Luschmann,[1,2,3] A. Faltermeier,[1,2] S. Weichselbaumer,[1,2,3] L. Koch,[1,2,3] G.B.P. Huber,[1,2] H.W. Schumacher,[4] N. Ubbelohde,[4] D. Reifert,[4] T. Scheller,[4] F. Deppe,[1,2,3] A. Marx,[1] S. Filipp,[1,2,3] M. Althammer,[1,2] R. Gross,[1,2,3] and H. Huebl[1,2,3,b)]

[1)] *Walther-Meißner-Institut, Bayerische Akademie der Wissenschaften, 85748 Garching, Germany*

[2)] *Physik-Department, Technische Universität München, 85748 Garching, Germany*

[3)] *Munich Center for Quantum Science and Technology (MCQST), 80799 Munich, Germany*

[4)] *Physikalisch-Technische Bundesanstalt, 38112 Braunschweig, Germany*

(Dated: December 13, 2021)

## I. X-RAY DIFFRACTION RESULTS OF NBTIN THIN FILM GROWN ON HF-DIPPED SI

We here present the results of x-ray diffraction experiments on the NbTiN thin films grown on HF-dipped Si-substrate in Fig. S1.

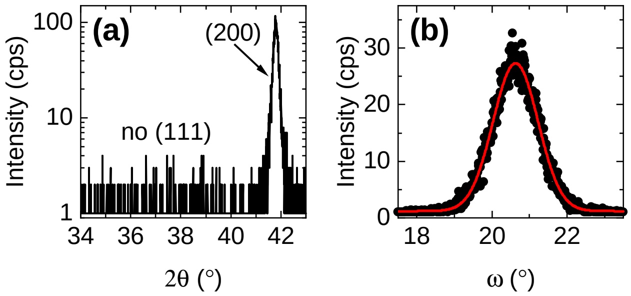


Figure S1. (a) $2\theta - \omega$ X-ray diffraction scan of the NbTiN film grown on HF-dipped (001) oriented Si. We observe a peak originating from a preferential (200) orientation of cubic NbTiN but no evidence for a preferred (111) orientation. (b) Rocking curve of the (200)-reflection. The red line indicates a gaussian fit to the raw data. We extract a full-width at half maximum (FWHM) of FWHM= $(1.19 \pm 0.01)^\circ$.

The $2\theta - \omega$ X-ray diffraction scan in Fig. S1(a) shows that the cubic NbTiN grows with a preferential (200) orientation on the Si (001) substrate. In Fig. S1(b), we fit the extracted rocking curve of the (200)-reflection to a gaussian fit and extract a full-width at half maximum (FWHM) of FWHM= $(1.19 \pm 0.01)^\circ$, which indicates a textured growth in agreement to literature (see Refs.1 and 2).
As the (200)-reflection peak could only be detected for a NbTiN film grown on the HF dipped Si-substrate, we infer that the removal of the native $SiO_2$-layer promotes the textured growth of cubic NbTiN.

[a)] manuel.mueller@wmi.badw.de

[b)] hans.huebl@wmi.badw.de

## II. RESONATOR QUALITY FACTORS

We here list the individual quality factors of the investigated resonators, which were used as a basis for the statistical mean values and standard deviations for the individual samples listed in Tab. 2 of the main text. Resonators that have been excluded from the statistical evaluation in the main text are marked with an asterisk *.

- $Nb_{70}Ti_{30}N$ on thermally oxidized Si

| Resonator | $f_r$ (GHz) | $Q$ ($\times10^3$) | $Q_{int}$ ($\times10^3$) | $Q_{ext}$($\times10^3$) |
|---|---|---|---|---|
| R1 | 5.256 | 15.0±0.1 | 26.2±0.1 | 35.4±0.1 |
| R2 | 5.398 | 8.0±0.1 | 9.4±0.1 | 54.9±1.0 |
| R3 | 5.525 | 6.7±0.4 | 10.0±0.4 | 19.8±4.2 |
| R4 | 5.689 | 6.1±0.5 | 7.7±0.6 | 29.4±1.4 |
| R5 | 5.769 | 10.4±0.1 | 12.9±0.1 | 54.3±0.1 |

- $Nb_{81}Ti_{19}N$ on thermally oxidized Si (PTB)

| Resonator | $f_r$ (GHz) | $Q$ ($\times10^3$) | $Q_{int}$ ($\times10^3$) | $Q_{ext}$($\times10^3$) |
|---|---|---|---|---|
| R1 | 4.485 | 16.5±0.1 | 29.7±0.2 | 37.4±0.1 |
| R2 | 4.584 | 8.5±0.1 | 15.8±0.1 | 18.4±0.1 |
| R3 | 4.697 | 13.2±0.8 | 16.6±0.8 | 66.0±2.8 |
| R4 | 4.793 | 10.2±0.1 | 33.1±0.3 | 14.7±0.1 |
| R5 | 4.870 | 10.0±0.1 | 11.3±0.2 | 89.4±0.4 |

- $Nb_{70}Ti_{30}N$ on pristine Si

| Resonator | $f_r$ (GHz) | $Q$ ($\times10^3$) | $Q_{int}$ ($\times10^3$) | $Q_{ext}$($\times10^3$) |
|---|---|---|---|---|
| R1 | 4.674 | 19.8±0.4 | 196.3±23.2 | 22.0±0.1 |
| R2 | 4.803 | 48.9±1.5 | 262.5±26.2 | 60.1±0.4 |
| R3 | 4.928 | 26.7±2.5 | 373.8±27.6 | 28.8±0.8 |
| R4 | 5.034 | 9.3±0.2 | 123.8±15.2 | 10.1±0.1 |
| R5 | 5.133 | 37.7±0.6 | 84.9±2.9 | 67.9±0.5 |

- $Nb_{70}Ti_{30}N$ on Si + HF dip

| Resonator | $f_r$ (GHz) | $Q$ ($\times10^3$) | $Q_{int}$ ($\times10^3$) | $Q_{ext}$($\times10^3$) |
|---|---|---|---|---|
| R1 | 4.672 | 84.7±1.4 | 215.2±9.0 | 139.7±0.1 |
| R2 | 4.806 | 61.0±0.1 | 152.2±5.3 | 101.9±0.1 |
| R3 | 4.924 | 84.3±0.6 | 207.8±3.8 | 141.9±0.1 |
| R4 | 5.026 | 69.4±2.3 | 161.7±12.0 | 121.5±0.1 |
| R5* | 5.133 | 17.9±0.1 | 50.6±0.1 | 27.9±0.1 |

## III. DETERMINATION OF THE SUPERCONDUCTING TRANSITION TEMPERATURE

To determine the superconducting transition temperature of our patterned NbTiN films, we continuously recorded the $S_{21}$-parameter at $f = 5$ GHz, while heating the sample at a constant rate of 2K/min. The result is shown in Fig. S2. We observe an abrupt drop in $S_{21}$, which we attribute to the transition of the sample to the normalconducting state at $T = 16.3 \pm 0.1$ K.

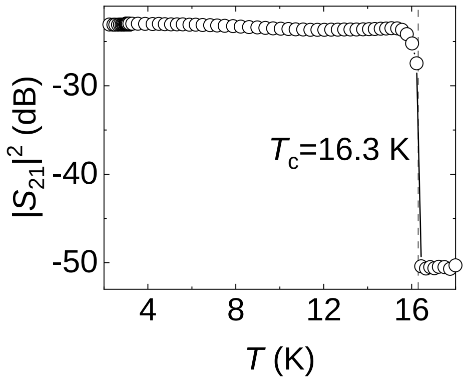


Figure S2. $S_{21}$-parameter recorded as function of $T$, while the resonator box was continuously heated at a rate of 2K/min

## IV. MICROWAVE CIRCUITRY FOR MK MEASUREMENTS

The cryostat used for the mK experiments was a Bluefors LD-400 dry dilution refrigerator. The used microwave circuitry ist depicted in Fig. S3. To suppress room temperature noise photons from reaching the sample under investigation, the input lines are attenuated by 86 dB within the various temperature stages. On the output side, we use a cryogenic circulator mounted on the mK stage. The outgoing signal is amplified by +40 dB with a cryogenic HEMT amplifier at the 4 K stage. Additionally, we measured $\approx 10.0$ dB cable losses from the microwave cables at the resonance frequency of the investigated resonator $f = f_{\mathrm{R1}} = 4.672$ GHz.

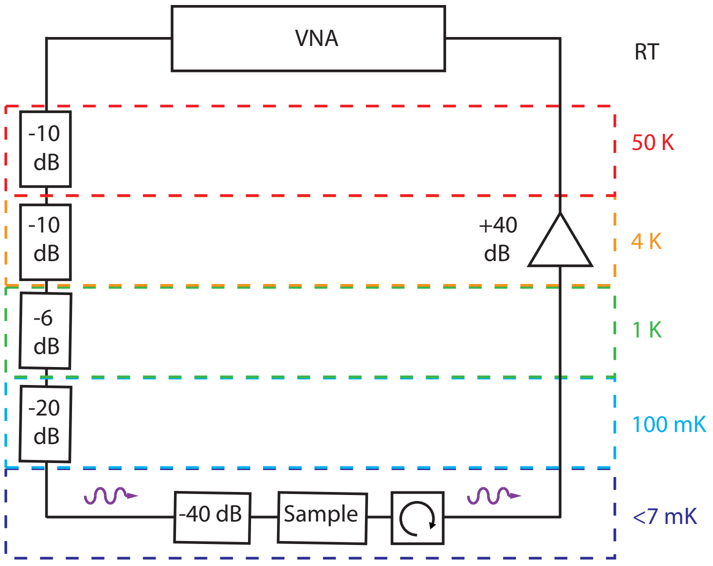


Figure S3. Microwave setup for mK experiments.

## V. PARTICIPATION RATIOS AND LOSS TANGENTS EXTRACTED FROM SIMULATION

The numerically calculated participation ratios of the four dielectric regions for our resonator layout are listed in Tab. S1. The total loss induced by TLS, $F\tan\delta^0_{\mathrm{TLS}} \approx 0.5 \cdot 10^{-6}$, is the sum of the listed $p_\mathrm{i}\tan(\delta_\mathrm{i})$.

| Resonator | metal-air (MA) | metal-substrate (MS) | substrate-air (SA) | substrate (S) |
|---|---|---|---|---|
| $p_\mathrm{i}$ | 3.4E-6 | 2.4E-4 | 1.6E-4 | 0.89 |
| $\tan(\delta_\mathrm{i})$ | 3.3E-3 | 2.7E-4 | 1.2E-3 | 2.6E-7 |
| $p_\mathrm{i}\tan(\delta_\mathrm{i})$ | 1.1E-8 | 6.5E-8 | 2E-7 | 2.3E-7 |
| $d_\mathrm{i}$ (nm) | 2 | 2 | 2 | 2 |
| $\epsilon_\mathrm{i}/\epsilon_0$ | 10 | 11.4 | 11.4 | 11.9 |

Table S1. Numerically calculated participation ratios $p_\mathrm{i}$, assumed loss tangents $\tan(\delta_\mathrm{i})$, layer thicknesses $d_\mathrm{i}$ and dielectric constants $\epsilon_\mathrm{i}/\epsilon_0$ of the four dielectric regions, following Ref. 3.

## REFERENCES

[1] H. Ge, Y.-R. Jin, and X.-H. Song, "High quality NbTiN films fabrication and rapid thermal annealing investigation," Chin. Phys. B **28**, 077402 (2019).
[2] L. Zhang, W. Peng, L. X. You, and Z. Wang, "Superconducting properties and chemical composition of NbTiN thin films with different thickness," Appl. Phys. Lett. **107**, 122603 (2015).
[3] A. Melville, G. Calusine, W. Woods, K. Serniak, E. Golden, B. M. Niedzielski, D. K. Kim, A. Sevi, J. L. Yoder, E. A. Dauler, and W. D. Oliver, "Comparison of dielectric loss in titanium nitride and aluminum superconducting resonators," Appl. Phys. Lett. **117**, 124004 (2020).
